# Supplementary material for: Enhancing structural resilience in healthcare through patient flow network
Source: arXiv:2410.06031 source file (2026-05-28)
Supplement: Supplementary file 1 [file supplementary.tex]

\documentclass{nature}

%% make sure you have the nature.cls and naturemag. bst files where
%% LaTeX can find them
\usepackage{subfigure}
\usepackage{array}
\usepackage{float}

\usepackage{graphicx}
\usepackage{amsmath}
\usepackage{amssymb}
\usepackage{lineno}
\linenumbers
\usepackage{caption}
\usepackage{booktabs}
\usepackage{multirow}
\usepackage{cite}
\usepackage{times}
\usepackage{color}
\usepackage{caption}
\usepackage{xurl}
\usepackage{adjustbox}
\usepackage{graphicx}
\usepackage{longtable}
\usepackage{docmute} 

\linespread{1}

\captionsetup[figure]{font=footnotesize}

\usepackage[dvipsnames]{xcolor}

\bibliographystyle{naturemag}

\title{Supplementary Information \\Patient flow networks absorb healthcare stress during pandemic crises}
\author{Lu Zhong${}^{1,2}$, Sen Pei${}^{3}$, Jianxi Gao${}^{1,2*}$}
\begin{document}

\maketitle

\subsection{Dataset.} Table \ref{SI_table_all_stats} presents essential statistics for the Healthjump datasets spanning from 2017 to 2022, including the total number of records and the proportion of valid data points among various age and race groups and health services. The categorization of health services is based on the ICD-10 diagnosis codes for Chronic Disease care and Acute Respiratory Illness care, as detailed in Table \ref{SI_table_service}. Valid data points are notably high at 99.8\% across age groups, moderate at 58.2\% across race groups, and markedly low, under 2\%, for both Chronic Disease care and Acute Respiratory Illness care.

To ensure each state is adequately represented in the dataset, we exclude those with insufficient data, defined as states where patient numbers are less than 0.1\% of the state population and include fewer than three regions. The excluded states are AK, CT, HI, MT, NE, NV, ND, RI, SD, and WI. Table \ref{SI_table_state} presents the statistics for the included states, details the characteristics of their patient flow networks, and the results of network absorptivity.

\subsection{Absorptivity for patient demographics.} Figure \ref{SI_race} illustrates the absorptivity rates for patient groups across various age groups. Children and the elderly exhibit lower absorptivity rates, recorded at $r=0.10$ and $r=0.16$, respectively, whereas the young and middle-aged groups show higher rates at $r=0.21$. Regarding racial demographics, Asian populations demonstrate the highest absorptivity at $r=0.69$, while White populations have the lowest at $r=0.24$.

\subsection{Absorptivity for healthcare services.} Regarding healthcare services (Fig. \ref{SI_network_service} and Fig.\ref{SI_service}), the absorptivity rates for Chronic Disease care remain relatively high and steady around $r=0.89$. The absorptivity rates for Acute Respiratory Illness care are lower and fluctuates round $r=0.40$ respectively.   However, these results are likely impacted by incomplete data, as less than 2\% of the dataset contains valid related ICD-10 codes, potentially limiting the comprehensiveness of the analysis.

\newpage
\begin{figure*}[h!]
\centering
\captionsetup{justification=justified}
\includegraphics[scale=1.0]{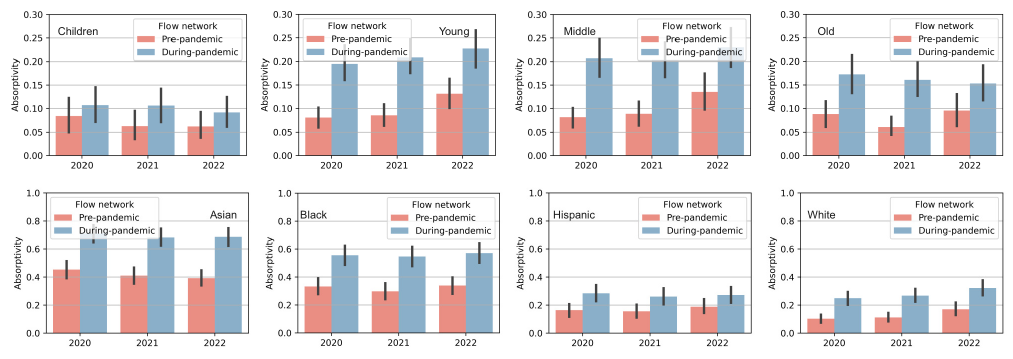}
\caption{\textbf{Absorptivity of different patient demographic.} We stratify the patient flow network based on demographic attributes, i.e., age groups and race and ethnicity groups.} 
\label{SI_race}
\end{figure*}

\clearpage
\begin{figure*}[h!]
\centering
\captionsetup{justification=justified}
\includegraphics[scale=0.9]{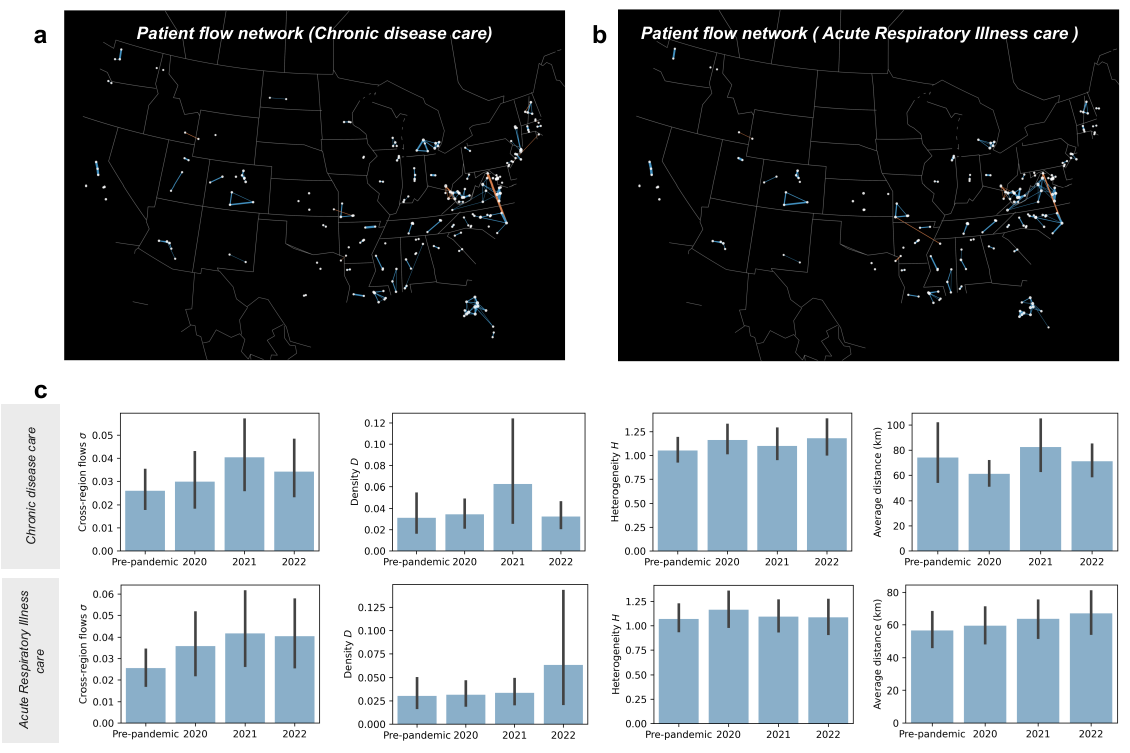}
\caption{\textbf{Absorptivity of different patient demographic.} We stratify the patient flow network based on demographic attributes, i.e., age groups and race and ethnicity groups.} 
\label{SI_network_service}
\end{figure*}

\begin{figure*}[h!]
\centering
\captionsetup{justification=justified}
\includegraphics[scale=0.9]{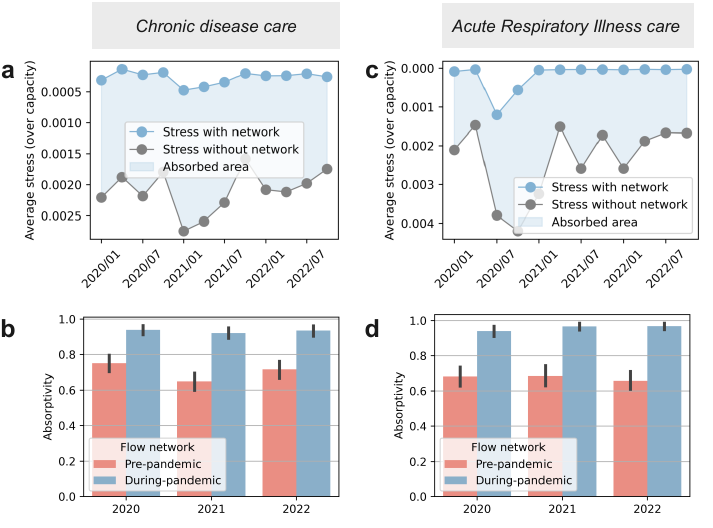}
\caption{\textbf{Absorptivity of different patient demographic.} We stratify the patient flow network based on demographic attributes, i.e., age groups and race and ethnicity groups.} 
\label{SI_service}
\end{figure*}

\newpage
\clearpage
{ % Don't forget to limit the scope
\scriptsize % Or other fontsize modifier
\begin{longtable}{|p{3cm}|p{1.5cm}|p{1.5cm}|p{1.5cm}|p{1.5cm}|p{1.5cm}|p{1.5cm}|p{1.5cm}|}
\hline
Number of records & 2017 & 2018 & 2019 & 2020 & 2021 & 2022 & Total\\ \hline
All services &24,030,514 & 26,625,274 & 30,423,281 & 32,829,805 & 40,327,414 & 43,327,540 &197,563,828 \\ \hline \hline
Children (Percent) & 14.1 \% &  13.9 \% &  13.3 \% &  11.0 \% &  11.6 \% &  11.7 \%  &12.4\%\\
Young (Percent) &24.6\% & 24.3\% & 24.2\% & 25.0\% & 24.7\% & 24.4\%  &24.5\% \\ 
Middle (Percent)&32.0\% &  31.6\% &  31.4\% &  32.2\% &  31.4\% &  30.6\%  &31.4\% \\ 
Old (Percent) & 29.3\% &  30.1\% &  31.1\% &  31.8\% &  32.3\% & 33.3\%  &31.5\% \\ \hline \hline
Asian (Percent)& 1.4 \% & 1.4 \% & 1.4\% & 1.3\% & 1.3 \% & 1.2\% &1.3\%\\ 
Black (Percent)& 8.1\% &  8.0\% &  8.1\% &  8.2\% & 7.8\% &  7.1\%  &7.8\%\\ 
Hispanic (Percent)&  9.8\% &  8.9\% &  8.2\% &  7.9\% &  8.2\% &  7.4\% &8.2\%  \\ 
white (Percent)& 42.1\% & 41.9\% & 41.3\% & 43.0\% & 41.2\% & 37.9\%  &40.9\% \\ \hline \hline
Chronic Disease Care (Percent) & 2.6\% & 2.3\% & 2.0\% & 1.8\% & 1.6 \% & 1.3 \% & 1.8\%\\ 
Acute Respiratory Illness Care (Percent) & 1.5\% & 1.3\% & 1.1\% & 1.3\% & 1.2\% & 1.0\% & 1.2\%\\ \hline \hline
\caption{Total number of electronic health records for the different patient groups in the Healthjump dataset.}
\label{SI_table_all_stats}
\end{longtable}}

\newpage
\clearpage
{ % Don't forget to limit the scope
\scriptsize % Or other fontsize modifier
\setlength\LTleft{-1.0cm}  % Change horizontal alignments
\setlength\LTright{4.0cm} % ... to make longtable wider
\begin{longtable}{|p{3.5cm}|p{3cm}|p{8cm}|p{2cm}|}
\hline
Services & Disease & Sub-disease & ICD-10 code  \\ \hline
\multirow{11}{*}{Chronic Disease Care} & Alzheimer’s disease &  Alzheimer’s disease &G30  \\ 
 \cline{2-4}  & Asthma & Asthma &  J45 - J46  \\ 
 \cline{2-4}  & Atherosclerosis & Atherosclerosis &I70  \\ 
 \cline{2-4} & Cancer & Malignant neoplasms of lip, oral cavity and pharynx; Malignant neoplasm of esophagus; Malignant neoplasm of stomach; Malignant neoplasms of colon, rectum and anus; Malignant neoplasms of liver \/ intrahepatic bile ducts; Malignant neoplasm of pancreas; Malignant neoplasm of larynx; Malignant neoplasms of trachea, bronchus and lung; Malignant melanoma of skin; Malignant neoplasm of breast; Malignant neoplasm of cervix uteri; Malignant neoplasms of corpus uteri and uterus, part unspecified; Malignant neoplasm of ovary; Malignant neoplasm of prostate; Malignant neoplasms of kidney and renal pelvis;Malignant neoplasm of bladder;	
Malignant neoplasms of meninges, brain and other parts of central nervous system; Hodgkin's disease; Non-Hodgkin's lymphoma; Leukemia; Multiple myeloma and immunoproliferative neoplasms; Other \/unspecified malignant neoplasms of lymphoid, hematopoietic \&related tissue; All other and unspecified malignant neoplasms & C00-C97   \\ 
 \cline{2-4} & Stroke (cerebrovascular diseases) &Stroke (cerebrovascular diseases)&  I60 - I69  \\ 
 \cline{2-4} & Chronic liver disease & Cirrhosis \& Alcoholic liver disease; Other chronic liver disease and cirrhosis& K70, K73 - K74   \\ 
 \cline{2-4} & Chronic Obstructive Pulmonary Disease (COPD) excluding Asthma &Bronchitis, chronic and unspecified;	
Emphysema;	
Other chronic lower respiratory diseases& J40 – J47  \\ 
 \cline{2-4}  & Diabetes & Diabetes & E10-E14  \\ 
 \cline{2-4} & {{Essential hypertension}} & {{Essential hypertension}} & I10, I12, I15  \\ 
 \cline{2-4} & {{Heart disease}} & 	
{{Acute rheumatic fever and chronic rheumatic heart diseases; Hypertensive heart disease; Hypertensive heart and renal disease; Acute myocardial infarction; Other acute ischemic heart diseases; Atherosclerotic cardiovascular disease, so described; All other forms of chronic ischemic heart disease; 	
Acute and subacute endocarditis; 	
Diseases of the pericardium and acute myocarditis; 	
Heart failure; All other forms of heart disease.}}& I00 - I09, I11, I13, 
I20 - I51  \\ 
 \cline{2-4} & Kidney disease (nephritis, nephrotic syndrome and nephrosis) &Acute nephritic / nephrotic syndrome; Chronic / unspecified nephritis and renal sclerosis; 	
Renal failure; Other disorders of kidney& N00 - N07, N17 - N19, 
N25 - N27  \\ 
 \cline{2-4} & Other cardiovascular/circulatory conditions & 	
Aortic aneurysm and dissection; Other diseases of arteries, arterioles and capillaries; Other disorders of circulatory system; & I71 - I78, I80 - I99  \\    \hline
\multirow{3}{*}{Acute Respiratory Illness Care} & COVID-19 &  &U07, U00, U09, U49, U50, U85\\ 
 \cline{2-4} &Acute upper respiratory infection& ~ & J00-J06 \\ 
 \cline{2-4}&Influenza and pneumonia& ~ & J09-J18 \\ 
 \cline{2-4}& Other acute lower respiratory infections & ~& J20-J22  \\ \hline
\caption{Services of concern, along with their sub-types and corresponding ICD-10 codes.}
\label{SI_table_service}
\end{longtable}}

\clearpage
\begingroup
  \scriptsize 
  \setlength\LTleft{-60pt}%
  \setlength\LTright{-60pt}%
  \centering 
\begin{longtable}{c|c|p{2cm}|p{1.5cm}|p{1.5cm}|p{1.5cm}|p{1.5cm}|p{1.5cm}|p{1.5cm}|p{1.5cm}}
\caption{Statistics of datasets across states and their patient networks. States (including AK, HI, ND, RI, SD, and MT) are not analyzed due to insufficient data with patient numbers less than 1\% of the population. }\\
\hline\hline
State &Period &Number of patients (Percentage of population)& Number of sub-regions (Total) & Percentage of cross-region flows&  \multicolumn{3}{c}{Topological measures}  &  \multicolumn{2}{|c}{Absorptivity}\\
\cline{6-10}  & & & &  & Average distance (km) &Density &Heterogenity &COVID-19 scenario & Identical scenario \\
\hline 
AL & pre-pandemic &  248,652(5.1\%) &  15(19) &  1.52\% & 137& 0.04& 1.02& 0.01 & 0.04 \\  
AL & during-pandemic &  319,176(6.6\%) &  15(19) &  1.62\% & 145& 0.06& 0.97& 0.01 & 0.06\\   \hline
AR & pre-pandemic &  161,014(5.4\%) &  12(14) &  1.26\% & 130& 0.17& 1.13&0.03 & 0.02 \\  
AR & during-pandemic &  270,159(9.0\%) &  12(14) &  3.38\% & 134& 0.25& 1.76& 0.09 & 0.09\\   \hline
AZ & pre-pandemic &  51,549(0.7\%) &  10(12) &  1.97\% & 68& 0.05& 1.5& 0.02 & 0.02  \\  
AZ & during-pandemic &  118,219(1.7\%) &  10(12) &  2.77\% & 119& 0.17& 1.52& 0.01 & 0.07\\   \hline
CA & pre-pandemic &  466,180(1.2\%) &  36(57) &  3.14\% & 71& 0.01& 1.65& 0.01 & 0.07\\  
CA & during-pandemic &  578,486(1.5\%) &  36(57) &  3.64\% & 74& 0.02& 2.2& 0.03 & 0.09\\   \hline
CO & pre-pandemic &  199,565(3.6\%) &  16(17) &  3.18\% & 90& 0.1& 1.48& 0.01 & 0.05\\  
CO & during-pandemic &  360,286(6.5\%) &  16(17) &  3.24\% & 114& 0.14& 1.67& 0.01 & 0.1\\   \hline
DE & pre-pandemic &  158,669(16.7\%) &  3(3) &  2.32\% & 64& 1.11& 0.25& 0.0 & 0.15\\  
DE & during-pandemic &  145,416(15.3\%) &  3(3) &  2.93\% & 64& 1.06& 0.28& 0.0 & 0.18\\   \hline
FL & pre-pandemic &  293,897(1.4\%) &  25(25) &  1.96\% & 54& 0.03& 1.95& 0.08 & 0.02 \\  
FL & during-pandemic &  511,707(2.5\%) &  25(25) &  2.51\% & 148& 0.2& 3.09& 0.19 & 0.04 \\   \hline
GA & pre-pandemic &  93,669(0.9\%) &  16(20) &  4.41\% & 85& 0.08& 1.75& 0.14 & 0.07 \\  
GA & during-pandemic &  122,219(1.2\%) &  16(20) &  4.1\% & 87& 0.08& 1.62& 0.24 & 0.08\\   \hline
ID & pre-pandemic &  15,455(0.9\%) &  3(7) &  0.05\% & 63& 0.02& 0.88& 0.05 & 0.08\\  
ID & during-pandemic &  31,221(1.8\%) &  3(7) &  0.19\% & 160& 0.02& 0.86& 0.51 & 0.0 \\   \hline
IL & pre-pandemic &  61,862(0.5\%) &  18(29) &  2.49\% & 65& 0.01& 1.11& 0.03 & 0.02\\  
IL & during-pandemic &  145,996(1.1\%) &  18(29) &  5.43\% & 78& 0.05& 1.84& 0.15 & 0.09\\   \hline
IN & pre-pandemic &  88,948(1.3\%) &  14(20) &  3.55\% & 74& 0.06& 1.9&0.04 & 0.03 \\  
IN & during-pandemic &  190,837(2.9\%) &  14(20) &  8.03\% & 75& 0.07& 1.68&0.23 & 0.15\\   \hline
IA & pre-pandemic &  20,079(0.6\%) &  12(25) &  2.72\% & 22& 0.01& 1.74&0.11 & 0.01 \\  
IA & during-pandemic &  31,751(1.0\%) &  12(25) &  4.94\% & 35& 0.04& 1.93&0.39 & 0.03 \\   \hline
KS & pre-pandemic &  32,813(1.1\%) &  12(19) &  0.37\% & 118& 0.04& 2.1& 0.02 & 0.0\\  
KS & during-pandemic &  44,972(1.5\%) &  12(19) &  0.81\% & 122& 0.09& 2.21&0.06 & 0.01 \\   \hline
KY & pre-pandemic &  12,821(0.3\%) &  19(27) &  1.49\% & 160& 0.05& 3.3& 0.03 & 0.01\\  
KY & during-pandemic &  34,780(0.8\%) &  19(27) &  4.53\% & 131& 0.11& 4.09&0.18 & 0.06 \\   \hline
LA & pre-pandemic &  223,456(4.8\%) &  13(13) &  1.41\% & 99& 0.16& 0.62&0.03 & 0.02 \\  
LA & during-pandemic &  280,591(6.0\%) &  13(13) &  2.77\% & 111& 0.32& 0.81&0.1 & 0.06 \\   \hline
ME & pre-pandemic &  25,813(1.9\%) &  3(11) &  4.98\% & 41& 0.04& 1.14& 0.85 & 0.05 \\  
ME & during-pandemic &  29,090(2.2\%) &  3(11) &  3.94\% & 63& 0.06& 1.48& 0.85 & 0.05 \\   \hline
MD & pre-pandemic &  130,026(2.2\%) &  13(13) &  2.08\% & 47& 0.12& 1.65& 0.0 & 0.05\\  
MD & during-pandemic &  139,238(2.3\%) &  13(13) &  2.4\% & 39& 0.15& 1.52& 0.0 & 0.06\\   \hline
MA & pre-pandemic &  19,444(0.3\%) &  12(18) &  6.21\% & 30& 0.02& 0.93&0.2 & 0.08 \\  
MA & during-pandemic &  34,785(0.5\%) &  12(18) &  9.5\% & 98& 0.04& 1.91& 0.42 & 0.2\\   \hline
MI & pre-pandemic &  131,895(1.3\%) &  15(20) &  10.14\% & 56& 0.04& 1.19&0.05 & 0.08 \\  
MI & during-pandemic &  254,381(2.6\%) &  15(20) &  8.78\% & 81& 0.09& 2.09&0.19 & 0.14 \\   \hline
MN & pre-pandemic &  47,024(0.9\%) &  7(16) &  3.75\% & 78& 0.05& 1.95& 0.03 & 0.06\\  
MN & during-pandemic &  98,481(1.8\%) &  7(16) &  5.53\% & 65& 0.06& 2.33& 0.1 & 0.16\\   \hline
MS & pre-pandemic &  147,907(4.9\%) &  10(12) &  1.73\% & 92& 0.1& 0.95& 0.09 & 0.03\\  
MS & during-pandemic &  185,691(6.2\%) &  10(12) &  2.99\% & 101& 0.16& 0.76&0.18 & 0.06 \\   \hline
MO & pre-pandemic &  41,504(0.7\%) &  12(25) &  3.02\% & 81& 0.02& 1.56& 0.05 & 0.05\\  
MO & during-pandemic &  58,040(1.0\%) &  12(25) &  3.14\% & 83& 0.04& 1.63&0.08 & 0.07 \\   \hline
NH & pre-pandemic &  9,430(0.7\%) &  5(9) &  5.85\% & 77& 0.11& 1.49&0.33 & 0.08 \\  
NH & during-pandemic &  26,907(2.0\%) &  5(9) &  4.17\% & 72& 0.14& 1.37& 0.31 & 0.09\\   \hline
NJ & pre-pandemic &  184,037(2.1\%) &  18(20) &  0.44\% & 37& 0.02& 1.8& 0.04 & 0.03\\  
NJ & during-pandemic &  222,418(2.5\%) &  18(20) &  0.51\% & 62& 0.03& 1.92&0.05 & 0.04 \\   \hline
NM & pre-pandemic &  2,982(0.1\%) &  3(13) &  0.52\% & 224& 0.03& 1.19&0.38 & 0.0 \\  
NM & during-pandemic &  3,359(0.2\%) &  3(13) &  0.66\% & 166& 0.01& 0.85& 0.92 & 0.0\\   \hline
NY & pre-pandemic &  44,954(0.2\%) &  27(51) &  5.14\% & 68& 0.02& 4.62& 0.04 & 0.03\\  
NY & during-pandemic &  197,593(1.0\%) &  27(51) &  4.32\% & 93& 0.08& 7.26& 0.12 & 0.08\\   \hline
NC & pre-pandemic &  644,225(6.3\%) &  20(20) &  1.92\% & 104& 0.19& 1.78&0.1 & 0.03 \\  
NC & during-pandemic &  845,225(8.3\%) &  20(20) &  2.91\% & 151& 0.39& 2.41&0.19 & 0.06 \\   \hline
OH & pre-pandemic &  90,992(0.8\%) &  17(29) &  3.06\% & 68& 0.04& 2.24&0.17 & 0.03 \\  
OH & during-pandemic &  139,812(1.2\%) &  17(29) &  6.16\% & 75& 0.05& 2.81&0.42 & 0.07 \\   \hline
OK & pre-pandemic &  42,992(1.1\%) &  11(17) &  5.89\% & 96& 0.02& 1.52&0.15 & 0.05 \\  
OK & during-pandemic &  87,145(2.2\%) &  11(17) &  8.04\% & 104& 0.04& 1.05&0.34 & 0.12 \\   \hline
OR & pre-pandemic &  56,276(1.4\%) &  6(10) &  3.27\% & 44& 0.04& 1.0& 0.05 & 0.08\\  
OR & during-pandemic &  70,187(1.7\%) &  6(10) &  3.53\% & 104& 0.04& 1.0& 0.08 & 0.11\\   \hline
PA & pre-pandemic &  156,775(1.2\%) &  14(46) &  0.04\% & 54& 0.0& 1.21& 0.0 & 0.0\\  
PA & during-pandemic &  190,173(1.5\%) &  14(46) &  0.16\% & 74& 0.01& 2.81& 0.0 & 0.01\\   \hline
SC & pre-pandemic &  162,532(3.3\%) &  9(10) &  1.31\% & 86& 0.19& 0.9& 0.02 & 0.03\\  
SC & during-pandemic &  214,085(4.3\%) &  9(10) &  2.9\% & 103& 0.33& 1.69& 0.02 & 0.11\\   \hline
TN & pre-pandemic &  187,285(2.8\%) &  15(15) &  5.78\% & 80& 0.15& 1.28& 0.11 & 0.09\\  
TN & during-pandemic &  349,438(5.3\%) &  15(15) &  6.43\% & 126& 0.26& 2.15& 0.17 & 0.15\\   \hline
TX & pre-pandemic &  256,682(0.9\%) &  34(50) &  1.84\% & 67& 0.01& 1.29& 0.01 & 0.03\\  
TX & during-pandemic &  457,854(1.6\%) &  34(50) &  2.4\% & 129& 0.03& 3.07&0.06 & 0.06 \\   \hline
UT & pre-pandemic &  446,158(14.7\%) &  7(7) &  3.43\% & 176& 0.3& 1.0&0.01 & 0.08 \\  
UT & during-pandemic &  508,198(16.7\%) &  7(7) &  3.93\% & 195& 0.53& 1.08&0.01 & 0.11 \\   \hline
VT & pre-pandemic &  1,600(0.3\%) &  3(9) &  1.07\% & 34& 0.03& 1.04& 0.36 & 0.02\\  
VT & during-pandemic &  1,683(0.3\%) &  3(9) &  1.44\% & 113& 0.03& 1.07&0.49 & 0.02 \\   \hline
VA & pre-pandemic &  156,950(1.9\%) &  27(28) &  7.53\% & 54& 0.09& 1.56&0.09 & 0.09 \\  
VA & during-pandemic &  226,931(2.7\%) &  27(28) &  9.7\% & 99& 0.16& 2.0& 0.28 & 0.19\\   \hline
WA & pre-pandemic &  108,628(1.5\%) &  8(14) &  0.98\% & 87& 0.02& 0.79& 0.01 & 0.02\\  
WA & during-pandemic &  134,158(1.8\%) &  8(14) &  1.11\% & 74& 0.04& 1.14& 0.02 & 0.03\\   \hline
WV & pre-pandemic &  122,013(6.7\%) &  18(22) &  6.23\% & 63& 0.08& 1.93& 0.22 & 0.12\\  
WV & during-pandemic &  139,590(7.6\%) &  18(22) &  7.2\% & 62& 0.1& 1.99& 0.28 & 0.15\\   \hline
WY & pre-pandemic &  4,869(0.8\%) &  8(13) &  2.66\% & 301& 0.04& 1.31&0.17 & 0.01\\  
WY & during-pandemic &  9,146(1.6\%) &  8(13) &  2.74\% & 281& 0.04& 1.09&0.62 & 0.03 \\   \hline
\hline
Total & pre-pandemic & 5351622 (1.6\%) &546 (805) &2.99\% 	 &86 &	0.09 & 1.49 &0.10 &0.04 \\ 
Total & during-pandemic &7809424 (2.3\%) &546 (805) & 3.88\% &105 &	0.14 &1.88  &0.21 & 0.08\\ \hline
\hline
\label{SI_table_state}
\end{longtable}
\endgroup

\end{document}
